# Supplementary material for: QuantBench: Benchmarking AI Methods for Quantitative Investment
Source: arXiv:2504.18600 source file (2025-04-24)
Supplement: Supplementary file 1 [file appendix.tex]

\twocolumn[ % This will make the content in the square brackets span two columns
   \centering
   \section*{Appendix}
   \vspace{\baselineskip} % Add a little space before continuing with two columns, adjust as needed
]

\section{Extended Related Works}

\section{Details on Dataset Preparations}

\section{Details on Model Implementations}

\section{Details on Evaluation Configurations and Metrics}

\section{Extended Experimental Results}
